# Supplementary material for: Evidence of Physiological Co-Modulation During Human-Animal Interaction: A Systematic Review
Source: arXiv:2510.10559 ancillary file (2025-10-12)
Supplement: Supplementary file 1 [file S11_Characteristics_of_Individual_Studies_Table.pdf]

Evidence of Physiological Co-Modulation During Human-Animal Interaction: A Systematic Review - Characteristics of Individual Studies Table (S11)

| Study                              | Animal specie(s) | Sample size | Interaction context | Physiological parameter                                    | Data Analysis Method Category      |
|------------------------------------|------------------|-------------|---------------------|------------------------------------------------------------|------------------------------------|
| (A. L. Baldwin et al., 2023)       | Horse            | < 10        | AAI                 | Cardiac Activity                                           | Time-Series Coupling               |
| (Baldwin et al., 2021)             | Horse            | < 10        | AAT                 | Cardiac Activity                                           | Time-Series Coupling               |
| (Buttner et al., 2015)             | Dog              | > 50        | Agonistic Sport     | Cortisol ( <i>dogs</i> )<br>Testosterone ( <i>humans</i> ) | Regression                         |
| (Byrne & Arnott, 2024)             | Dog              | > 20        | Companionship       | Cardiac Activity                                           | Regression                         |
| (Callara et al., 2024)             | Horse            | = 20        | AAI                 | Cardiac Activity                                           | Time-Series Coupling               |
| (Friend et al., 2023)              | Horse            | < 10        | AAT                 | Cardiac Activity<br>Cortisol                               | Discrete-Time Correlation Analysis |
| (Gnanadesikan, King, et al., 2024) | Dog              | > 50        | Companionship       | Oxytocin                                                   | Regression                         |
| (Grigg et al., 2022)               | Dog              | > 30        | Companionship       | Cardiac Activity                                           | Discrete-Time Correlation Analysis |
| (Guidi et al., 2016)               | Horse            | < 10        | AAI                 | Cardiac Activity                                           | Time-Series Coupling               |
| (Handlin et al., 2012)             | Dog              | = 10        | Companionship       | Cortisol<br>Oxytocin                                       | Discrete-Time Correlation Analysis |
| (Harvie et al., 2021)              | Dog              | > 60        | Companionship       | Cardiac Activity<br>Cortisol                               | Regression                         |
| (Hockenhull et al., 2015)          | Horse            | > 10        | Non-Agonistic Sport | Cardiac Activity                                           | Discrete-Time Correlation Analysis |
| (Holder et al., 2024)              | Dog              | < 10        | Companionship       | Cardiac Activity                                           | Time-Series Coupling               |
| (Janczarek et al., 2013)           | Horse            | < 10        | Non-Agonistic Sport | Cardiac Activity                                           | Discrete-Time Correlation Analysis |
| (Jones & Josephs, 2006)            | Dog              | > 80        | Agonistic Sport     | Cortisol ( <i>dogs</i> )<br>Testosterone ( <i>humans</i> ) | Regression                         |
| (Kang & Yun, 2016)                 | Horse            | > 20        | Agonistic Sport     | Cortisol                                                   | Discrete-Time Correlation Analysis |

| Study                   | Animal species | Sample size | Interaction context | Physiological parameter                                                                                                                                                                                                                                                  | Data Analysis Method Category      |
|-------------------------|----------------|-------------|---------------------|--------------------------------------------------------------------------------------------------------------------------------------------------------------------------------------------------------------------------------------------------------------------------|------------------------------------|
| (Katayama et al., 2019) | Dog            | > 30        | Companionship       | Cardiac Activity                                                                                                                                                                                                                                                         | Time Series Correlation            |
| (Koskela et al., 2024)  | Dog            | > 20        | Companionship       | Cardiac Activity                                                                                                                                                                                                                                                         | Regression                         |
| (Lanata et al., 2016)   | Horse          | < 10        | AAI                 | Cardiac Activity                                                                                                                                                                                                                                                         | Time-Series Coupling               |
| (Lanata et al., 2017)   | Horse          | < 10        | AAI                 | Cardiac Activity                                                                                                                                                                                                                                                         | Time-Series Coupling               |
| (McDuffee et al., 2024) | Horse          | < 10        | AAI                 | Cardiac Activity<br>Cortisol<br>Oxytocin                                                                                                                                                                                                                                 | Time-Series Correlation            |
| (Naber et al., 2025)    | Horse          | < 10        | AAT                 | Cardiac Activity<br>Cortisol                                                                                                                                                                                                                                             | Discrete-Time Correlation Analysis |
| (Nagasawa et al., 2015) | Dog<br>Wolf    | > 30        | Companionship       | Oxytocin                                                                                                                                                                                                                                                                 | Discrete-Time Correlation Analysis |
| (Nagasawa et al., 2023) | Dog            | > 20        | Companionship       | Cardiac Activity                                                                                                                                                                                                                                                         | Time Series Correlation            |
| (Nomoto et al., 2024)   | Dog            | < 10        | Companionship       | Breath Rithm                                                                                                                                                                                                                                                             | Regression                         |
| (Rankins et al., 2025a) | Horse          | < 10        | AAI                 | Cardiac Activity                                                                                                                                                                                                                                                         | Discrete-Time Correlation Analysis |
| (Ren et al., 2024)      | Dog            | > 10        | Companionship       | EEG                                                                                                                                                                                                                                                                      | Time-Series Coupling               |
| (Rişvanli et al., 2025) | Horse          | = 40        | Agonistic Sport     | Hormones:<br>Cortisol, ACTH,<br>$\beta$ -endorphin,<br>epinephrine,<br>norepinephrine, $T_3$ ,<br>$T_4$<br>Biochemical:<br>$Na$ , $K$ , CREA,<br>urea, TP, ALB, Mg,<br>AP, CK, ALT, AST<br>Haematological:<br>WBC, RBC, HGB,<br>HCT, MCV, MCH,<br>MCHC, PLT, LYM,<br>GRA | Discrete-Time Correlation Analysis |
| (Ryan et al., 2019)     | Dog            | > 20        | Companionship       | Cortisol<br>Cg A                                                                                                                                                                                                                                                         | Discrete-Time Correlation Analysis |
| (Schöberl et al., 2012) | Dog            | > 20        | Companionship       | Cortisol                                                                                                                                                                                                                                                                 | Discrete-Time Correlation Analysis |

| Study                   | Animal species | Sample size | Interaction context | Physiological parameter | Data Analysis Method Category      |
|-------------------------|----------------|-------------|---------------------|-------------------------|------------------------------------|
| (Schöberl et al., 2017) | Dog            | > 130       | Companionship       | Cortisol                | Discrete-Time Correlation Analysis |
| (Strzelec et al., 2013) | Horse          | > 30        | Agonistic Sport     | Cortisol                | Discrete-Time Correlation Analysis |
| (Sundman et al., 2019)  | Dog            | > 50        | Agonistic Sport     | Cortisol                | Regression                         |
| (Wienhold et al., 2025) | Horse          | < 10        | AAT                 | Cardiac Activity        | Time-Series Coupling               |
| (Wojtaś et al., 2020)   | Dog            | > 40        | Working Animals     | Cortisol                | Discrete-Time Correlation Analysis |
| (Wojtaś et al., 2022)   | Dog<br>Cat     | > 20        | Companionship       | Cortisol                | Discrete-Time Correlation Analysis |
| (Yorke et al., 2013)    | Horse          | < 10        | AAT                 | Cortisol                | Cross-Correlation                  |

#### Characteristics of Individual Studies Table:

The table presents main characteristics of each study.

The full names of all abbreviations, as well as definitions for each characteristic, are listed in the Supplementary Document S4. Additionally, a brief narrative summary of each study is available in the Supplementary Document S12.
