# Supplementary material for: Evidence of Physiological Co-Modulation During Human-Animal Interaction: A Systematic Review
Source: arXiv:2510.10559 ancillary file (2025-10-12)
Supplement: Supplementary file 3 [file S13_Individual_Studies_Results_Table.pdf]

# Evidence of Physiological Co-Modulation During Human-Animal Interaction: A Systematic Review - Individual Studies Results Table (S13)

| Name                               | Physiological parameters       | Analysis description                                                                                                                                                                              | Data Analysis Method Category      | Outcome     |
|------------------------------------|--------------------------------|---------------------------------------------------------------------------------------------------------------------------------------------------------------------------------------------------|------------------------------------|-------------|
| (A. L. Baldwin et al., 2023)       | Cardiac Activity               | Peak frequency analysis after FFT                                                                                                                                                                 | Time-Series Coupling               | Significant |
| (Baldwin et al., 2021)             | Cardiac Activity               | Fast Fourier Transform (FFT) used to identify Heart Rate Variability (HRV) frequency peaks. Coupling was defined as matching HRV frequency peaks (to 3–4 decimal places) between horse and human. | Time-Series Coupling               | Significant |
| (Buttner et al., 2015)             | Cortisol<br>Testosterone       | Pearson correlation Structural equation modelling (SEM) to test:<br>human Cortisol Variation influence on dog Cortisol Variation;<br>dog Cortisol Variation influence on human Cortisol Variation | Regression                         | Significant |
| (Byrne & Arnott, 2024)             | Cardiac Activity               | Linear Regression: human heart rate variation influence on dog heart rate variation.                                                                                                              | Regression                         | Significant |
| (Callara et al., 2024)             | Cardiac Activity               | Directed Coherence (DC - directional physiological coupling in the frequency domain).                                                                                                             | Time-Series Coupling               | Significant |
| (Friend et al., 2023)              | Cardiac Activity;<br>Cortisol; | Spearman correlation                                                                                                                                                                              | Discrete-Time Correlation Analysis | Partial     |
| (Gnanadesikan, King, et al., 2024) | Oxytocin                       | Bayesian model: fit univariate models using dog's Area Under the Curve (AUCi) as the outcome variable and child's Area Under the Curve (AUCi) as a predictor variable                             | Regression                         | Partial     |
| (Grigg et al., 2022)               | Cardiac Activity               | Pearson Correlation                                                                                                                                                                               | Discrete-Time Correlation Analysis | Partial     |
| (Guidi et al., 2016)               | Cardiac Activity               | Dynamic Time Warping                                                                                                                                                                              | Time-Series Coupling               | Significant |
| (Handlin et al., 2012)             | Cortisol;<br>Oxytocin;         | Spearman correlation                                                                                                                                                                              | Discrete-Time Correlation Analysis | Partial     |

| Name                      | Physiological parameters                    | Analysis description                                                                                                                                      | Data Analysis Method Category      | Outcome     |
|---------------------------|---------------------------------------------|-----------------------------------------------------------------------------------------------------------------------------------------------------------|------------------------------------|-------------|
| (Harvie et al., 2021)     | Cardiac Activity;<br>Cortisol;              | Heart Rate difference: calculated as the variation between the experimental timepoints.                                                                   | Regression                         | Absent      |
| (Hockenhull et al., 2015) | Cardiac Activity                            | Spearman's Rank Order Correlations of Heart Rate time series                                                                                              | Discrete-Time Correlation Analysis | Partial     |
| (Holder et al., 2024)     | Cardiac Activity                            | Pearson correlation; Dynamic time-warping methodology,                                                                                                    | Time-Series Coupling               | Absent      |
| (Janczarek et al., 2013)  | Cardiac Activity                            | Pearson Correlation                                                                                                                                       | Discrete-Time Correlation Analysis | Partial     |
| (Jones & Josephs, 2006)   | Cortisol (dogs);<br>Testosterone (humans);  | Linear Regression                                                                                                                                         | Regression                         | Significant |
| (Kang & Yun, 2016)        | Cortisol                                    | Pearson Correlation                                                                                                                                       | Discrete-Time Correlation Analysis | Partial     |
| (Katayama et al., 2019)   | Cardiac Activity                            | Calculation of Cross-Correlation between cortisol levels (lag-zero).                                                                                      | Time Series Correlation            | Significant |
| (Koskela et al., 2024)    | Cardiac Activity                            | Spearman correlation<br>Multivariate linear Regression.                                                                                                   | Regression                         | Significant |
| (Lanata et al., 2016)     | Cardiac Activity                            | Coherence (Magnitude Squared Coherence - MSC, Mean Phase Coherence - MPC); Dynamic time warping;                                                          | Time-Series Coupling               | Significant |
| (Lanata et al., 2017)     | Cardiac Activity                            | Nonlinear coupling and similarity measures: Cross-Entropy; Cross information Potential; Correntropy coefficient;                                          | Time-Series Coupling               | Significant |
| (McDuffee et al., 2024)   | Cardiac Activity;<br>Cortisol;<br>Oxytocin; | Bland-Altman plots of Heart Rate Variability (HRV) indices Sympathetic Nervous System (SNS) to Parasympathetic Nervous System (PNS) ratio (SNS/PNS ratio) | Time-Series Correlation            | Significant |
| (Naber et al., 2025)      | Cardiac Activity;<br>Cortisol;              | Spearman correlation                                                                                                                                      | Discrete-Time Correlation Analysis | Significant |

| Name                    | Physiological parameters               | Analysis description                                                                                                                                                                              | Data Analysis Method Category      | Outcome     |
|-------------------------|----------------------------------------|---------------------------------------------------------------------------------------------------------------------------------------------------------------------------------------------------|------------------------------------|-------------|
| (Nagasawa et al., 2015) | Oxytocin                               | Correlation (not specified)                                                                                                                                                                       | Discrete-Time Correlation Analysis | Significant |
| (Nagasawa et al., 2023) | Cardiac Activity                       | Correlation coefficients (not specified)                                                                                                                                                          | Time Series Correlation            | Significant |
| (Nomoto et al., 2024)   | Breath Rhythm                          | Generalized Linear Mixed Model (GLMM) to test the effect of human breathing on dog breathing. Fixed factors: human delta-breathing-interval (delta-BI), condition. Random effect: dog-owner pair. | Regression                         | Significant |
| (Rankins et al., 2025a) | Cardiac Activity                       | ANOVA for group comparisons, Pearson between human/horse indices + Bonferroni                                                                                                                     | Discrete-Time Correlation Analysis | Absent      |
| (Ren et al., 2024)      | EEG                                    | Interbrain correlation (Pearson correlation of EEG power). Generalized Partial Directed Coherence (GPDC) – directionality of coupling. Theta/Beta Ratio (TBR) – attention index                   | Time-Series Coupling               | Significant |
| (Rıřvanlı et al., 2025) | Hormones, Biochemical, Haematological. | Spearman correlation for horse-rider parameters, separate analysis for winners/losers .                                                                                                           | Discrete-Time Correlation Analysis | Partial     |
| (Ryan et al., 2019)     | Cortisol; Cg A;                        | Pearson Correlation                                                                                                                                                                               | Discrete-Time Correlation Analysis | Significant |
| (Schöberl et al., 2012) | Cortisol                               | Pearson Correlation                                                                                                                                                                               | Discrete-Time Correlation Analysis | Absent      |
| (Schöberl et al., 2017) | Cortisol                               | Spearman Correlation of individual coefficients of variance of cortisol (iCVs)                                                                                                                    | Discrete-Time Correlation Analysis | Absent      |
| (Strzelec et al., 2013) | Cortisol                               | Pearson Correlation                                                                                                                                                                               | Discrete-Time Correlation Analysis | Partial     |
| (Sundman et al., 2019)  | Cortisol                               | Generalised Linear Model                                                                                                                                                                          | Regression                         | Significant |

| Name                    | Physiological parameters | Analysis description                                  | Data Analysis Method Category      | Outcome     |
|-------------------------|--------------------------|-------------------------------------------------------|------------------------------------|-------------|
| (Wienhold et al., 2025) | Cardiac Activity         | cross-wavelet power analyses                          | Time-Series Coupling               | Significant |
| (Wojtaś et al., 2020)   | Cortisol                 | Spearman Correlation                                  | Discrete-Time Correlation Analysis | Significant |
| (Wojtaś et al., 2022)   | Cortisol                 | Spearman Correlation                                  | Discrete-Time Correlation Analysis | Partial     |
| (Yorke et al., 2013)    | Cortisol                 | Zero-lag Cross-Correlation for each child-horse pair. | Cross-Correlation                  | Significant |

**Individual Studies Results Table:**

The table displays results for each retrieved study, summarizing the measured parameters, analysis methods, and outcomes for each included study. A more detailed narrative description of each study and its results is available as a Supplementary Material (see: Supplementary Document S12).
