# Supplementary material for: Evidence of Physiological Co-Modulation During Human-Animal Interaction: A Systematic Review
Source: arXiv:2510.10559 ancillary file (2025-10-12)
Supplement: Supplementary file 4 [file S1_Search_Strategy_Document.pdf]

# Evidence of Physiological Co-Modulation During Human-Animal Interaction: A Systematic Review - Search Strategy Document (S1)

---

The following databases have been separately consulted:

- PubMed (via NCBI interface; coverage: 1946–present, as per MEDLINE)
- EMBASE (via Elsevier; coverage: 1947–present)
- Scopus (via Elsevier; coverage: 1788–present, citation data from 1970)
- Google Scholar (via web interface; coverage not explicitly defined)
- Animal Studies Repository (via institutional repository interface; coverage: repository active since 2014, includes archival material).

No study registries have been consulted. Additionally, the research tool "Consensus app" (<https://consensus.app/>) was screened. Although not a traditional bibliographic database, the Consensus App was included to enhance sensitivity and identify potentially relevant studies not indexed in standard databases. Its use was exploratory and the top-ranked results were screened with the same eligibility criteria.

Consensus App was interrogated with prompts written in natural language and structured as questions, with whom this tool best performs. The search was conservatively limited to the first twenty results, due to the fact that, on average, less than 10 results of the output of this tool are properly related to the question asked.

Citation searching was performed for each eligible entry identified through database and tool interrogation (via Google Scholar web interface).

In performing citation search a filter for papers published after 2024 was applied in order to limit the inclusion to the most recent advances on the

subject. No other restrictions were applied regarding the year of publication. Additionally, the ‘related articles’ function in the Google Scholar web interface was performed, for each eligible entry identified through database and tool interrogation, to identify potentially relevant studies.

To identify additional relevant studies, faculty members, postdoctoral researchers, and research fellow affiliated with the CoMPBioS research group from the Department of Information engineering and related units at the University of Florence, as well as external collaborators and affiliated researchers working with CoMPBioS on related projects, were contacted and invited to share any publications they were aware of that met the inclusion criteria of this review.

For each database separate searches for the following eight keywords boolean combinations have been run:

- "human animal interaction" AND "physiological measures"
- "human animal interaction" AND "EEG"
- "human animal interaction" AND "PPG"
- "human animal interaction" AND "fNIRS"
- "human animal interaction" AND "heart rate"
- "human animal interaction" AND "oxytocin"
- "human animal interaction" AND "cortisol"
- "human animal interaction" AND "breath"

As an example, the following query was entered directly into the search bar of each database:

"human animal interaction" AND "EEG"

Separate searches were conducted for each keyword combination to facilitate workload distribution, maintain syntactic clarity, and ensure reproducibility. This approach also allowed for better control over search results,

57 as some databases handle complex Boolean logic differently, and minimized  
58 the risk of retrieving irrelevant records due to overly broad Boolean logic.

59 Consensus App was interrogated with the following prompts (this tool  
60 best performs with prompts written in natural language and structured as  
61 questions):

- 62 • "are there publications which correlate animal and human EEG mea-  
63 sures in the context of human-animal interaction?"
- 64 • "are there publications which correlate animal and human PPG mea-  
65 sures in the context of human-animal interaction?"
- 66 • "are there publications which correlate animal and human fNIRS mea-  
67 sures in the context of human-animal interaction?"
- 68 • "are there publications which correlate animal and human heart rate  
69 measures in the context of human-animal interaction?"
- 70 • "are there publications which correlate animal and human oxytocin  
71 measures in the context of human-animal interaction?"
- 72 • "are there publications which correlate animal and human cortisol mea-  
73 sures in the context of human-animal interaction?"
- 74 • "are there publications which correlate animal and human breath mea-  
75 sures in the context of human-animal interaction?".

76 The screening on Consensus App was conservatively limited to the first  
77 twenty results, due to the fact that, on average, less than 10 results of the  
78 output of this tool are properly related to the question asked.

79 The term "correlate" was used in a broad sense to capture studies that simul-  
80 taneously measured physiological signals in humans and animals during inter-  
81 action and performed any quantitative analysis assessing their co-modulation  
82 (e.g., time-series coupling, correlation).

83  
84 The first keywords combination ("human animal interaction" AND "phys-  
85 iological measures") and the first prompt ("are there publications which cor-  
86 relate animal and human physiological measures measures in the context of  
87 human-animal interaction?") were strictly based on the "Intervention" fea-  
88 ture of the PICO for this review (Simultaneous measurement of physiological

parameters during human-animal interaction).

The term "physiological" has been interpreted as "*physical quantities such as temperature, cardiac activity, blood pressure, chemistry values in the blood and urine, enzymes, and proteins*" (Frize, 2014).

The choice of the composite keyword "human animal interaction" was based on its extensive use in the context of Animal Assisted Therapy (AAT) and Intervention (AAI) literature.

The decision to restrict the keyword strategy to the "Intervention" component of the PICO was aimed at maximizing the coverage of the search, in order to capture a wider spectrum of potentially relevant studies.

Then, in order to enhance the sensitivity of the search, additional queries were performed using more specific alternatives to the general term "physiological parameters", namely the most frequently used physiological signals in current human-animal interaction research (EEG, PPG, fNIRS, heart rate, oxytocin, cortisol, breath).

To ensure methodological rigour and data availability, papers that had not been peer reviewed, master or bachelor thesis, unpublished papers, conference papers and papers written in languages other than English have been excluded.

In performing citation search a filter for papers published after 2024 was applied in order to limit the inclusion to the most recent advances on the subject. No other restrictions were applied regarding the year of publication. All searches were conducted manually by entering each Boolean keyword combination directly into the search bar of each database's web interface, without the use of advanced syntax, field tags, or controlled vocabulary. No additional filters (e.g., language, date, species) were applied, except for limiting results to the category "article". This restriction was applied to exclude grey literature and ensure inclusion of peer-reviewed primary research, in line with the eligibility criteria of this review.

No search strategies from other literature reviews were adapted, reused or updated in this search.

All databases and tools were last consulted by the first reviewer on the 17th of July 2025 in an additional final screening, with the aim of checking for wrongly ignored entries (which were not found).

Finally, all databases were last checked between the 1 and 5 of August 2025 by the second reviewer.

Citing and related papers were last consulted by the first reviewer on the

18th of July 2025 in an additional final screening, with the aim of checking for wrongly ignored entries (which were not found). Finally, citing and related papers were last checked between the 1 and 5 of August 2025 by the second reviewer.

This search strategy has not undergone any peer review process.

Titles for a total of 1179 records were screened (1059 from bibliographic databases: Animal studies repository ( $n = 64$ ), Cochrane ( $n = 5$ ), EMBase ( $n = 303$ ), PubMed ( $n = 93$ ), Google Scholar ( $n = 400$ ), Scopus ( $n = 194$ ); and 120 from the Consensus App). Titles that clearly referred exclusively to behavioural measures, or to physiological parameters measured in either humans or animals only, were excluded.

Titles that did not explicitly mention physiological measures in both species, but also did not clearly indicate behavioural or single-species data, were further assessed at the abstract level.

Only studies that reported physiological measurements collected simultaneously in both humans and animals during interaction were included.

A total of 22 entries (14 from databases, 3 from consensus, 5 shared by the individuals who had been invited to contribute) were included.

Citation searching was performed for each eligible entry identified as well as interrogation of the 'related articles' tools in Google Scholar.

Additional 49 entries (7 from citation searching, 42 from 'related articles') that reported physiological measurements collected simultaneously in both humans and animals were included.

Search results have been saved in a Zotero collection (see: Supplementary File S2). All title-screened entries are stored in the folder "title screened", divided in subfolders that identify entries from each database, from citation searching, from related articles search and shared entries. All text-screened entries are stored in the folder "text screened", divided in subfolders that identify entries from each database, from citation searching, from related articles search and shared entries.

Three studies were excluded for being technological feasibility studies with no representative sample ( $n \leq 2$ ) and did not focus on analysis of measured data (Foster et al., 2018; Patel et al., 2021; Holder et al., 2022). One conference paper (Holder et al., 2023), one non-peer-reviewed report (Gehrke, 2010) and one paper written in Japanese (Kikusui, 2017) were excluded due

165 to aforementioned eligibility criteria. Twenty-four papers were excluded be-  
 166 cause they did not directly and quantitatively compare physiological signals  
 167 from human and animal subjects (Kotrschal et al., 2009; Clark et al., 2020;  
 168 Hama et al., 1996; Meinert et al., 2019; Merckes et al., 2014; Müller-Klein  
 169 et al., 2024; Pirrone et al., 2017; Yoon and Jung, 2025; Akiyama and Ohta,  
 170 2021; Ille et al., 2013, 2014; Handlin et al., 2011; Haubenhofner and Kirchen-  
 171 gast, 2007; Von Lewinski et al., 2013; Peeters et al., 2013; Ayala et al., 2021;  
 172 Crews, 2009; Gnanadesikan et al., 2024; Malinowski et al., 2018; Munsters  
 173 et al., 2012; Odendaal and Meintjes, 2003; Odendaal, 2000; Haubenhofner  
 174 et al., 2005; Dreschel and Granger, 2005).

175 Thirty-seven studies that simultaneously measured physiological parameters  
 176 in both humans and animals during an interaction and performed a co-  
 177 modulation statistical analysis (defined as any quantitative analysis assessing  
 178 their co-modulation) between the measured human and animal physiological  
 179 signals, were included.

180

181 No automation processes have been used for the deduplication. A list of  
 182 the eligible records has been constantly updated during the search, so that  
 183 pre-identified eligible records were not recorded more than once.

184

## References

- Akiyama, J., Ohta, M., 2021. Hormonal and Neurological Aspects of Dog Walking for Dog Owners and Pet Dogs. *Animals* doi:10.3390/ani11092732.
- Ayala, M.D., Carrillo, A., Iniesta, P., Ferrer, P., 2021. Pilot Study of the Influence of Equine Assisted Therapy on Physiological and Behavioral Parameters Related to Welfare of Horses and Patients. *Animals* doi:10.3390/ani11123527.
- Clark, S.D., Smidt, J.M., Bauer, B.A., 2020. Therapy Dogs' and Handlers' Behavior and Salivary Cortisol During Initial Visits in a Complex Medical Institution: A Pilot Study. *Front. Vet. Sci.* doi:10.3389/fvets.2020.564201.
- Crews, D., 2009. The Bond Between a Horse and a Human. *Nat Prec* doi:10.1038/npre.2009.3454.1.
- Dreschel, N.A., Granger, D.A., 2005. Physiological and behavioral reactivity to stress in thunderstorm-phobic dogs and their caregivers. *Applied Animal Behaviour Science* doi:10.1016/j.applanim.2005.04.009.

- Foster, M., Beppler, E., Holder, T., Dieffenderfer, J., Erb, P., Everette, K., Gruen, M., Somers, T., Evans, T., Daniele, M., Roberts, D.L., Bozkurt, A., 2018. A System for Assessment of Canine-Human Interaction during Animal-Assisted Therapies, in: 2018 40th Annual International Conference of the IEEE Engineering in Medicine and Biology Society (EMBC), IEEE, Honolulu, HI. doi:10.1109/EMBC.2018.8513384.
- Frize, M., 2014. Measuring Physiological Variables in Humans. Springer International Publishing, Cham. doi:10.1007/978-3-031-01657-8\_2.
- Gehrke, E.K., 2010. The horse-human heart connection: Results of studies using heart rate variability. NAHRA's Strides, Spring .
- Gnanadesikan, G.E., Carranza, E., King, K.M., Flyer, A.C., Ossello, G., Smith, P.G., Steklis, N.G., Steklis, H.D., Connelly, J.J., Barnett, M., Gee, N., Tecot, S., MacLean, E.L., 2024. Glucocorticoid response to naturalistic interactions between children and dogs. *Hormones and Behavior* doi:10.1016/j.yhbeh.2024.105523.
- Hama, H., Yogo, M., Matsuyama, Y., 1996. Effects of stroking horses on both humans' and horses' heart rate responses<sup>1</sup>. *Jpn Psychol Res* doi:10.1111/j.1468-5884.1996.tb00009.x.
- Handlin, L., Hydbring-Sandberg, E., Nilsson, A., Ejdebäck, M., Jansson, A., Uvnäs-Moberg, K., 2011. Short-Term Interaction between Dogs and Their Owners: Effects on Oxytocin, Cortisol, Insulin and Heart Rate—An Exploratory Study. *Anthrozoös* doi:10.2752/175303711X13045914865385.
- Haubenhofer, D., Möstl, E., Kirchengast, S., 2005. Cortisol concentrations in saliva of humans and their dogs during intensive training courses in animal-assisted therapy. *Wiener Tierärztliche Monatsschrift* .
- Haubenhofer, D.K., Kirchengast, S., 2007. 'Dog Handlers' and Dogs' Emotional and Cortisol Secretion Responses Associated with Animal-Assisted Therapy Sessions. *Soc Animals* doi:10.1163/156853007x187090.
- Holder, T., Rahman, M., Summers, E., Roberts, D., Wong, C.W., Bozkurt, A., 2022. Contact-Free Simultaneous Sensing of Human Heart Rate and Canine Breathing Rate for Animal Assisted Interactions, in: Proceedings of the Ninth International Conference on Animal-Computer Interaction, ACM, Newcastle-upon-Tyne United Kingdom. doi:10.1145/3565995.3566039.
- Holder, T.R.N., Nichols, C., Summers, E., Roberts, D.L., Bozkurt, A., 2023. Towards a Multimodal Synchronized System for Quantifying Psychophysiological States in Canine Assisted Interactions, in: The Tenth International Conference on Animal-Computer Interaction, ACM, Raleigh NC USA. doi:10.1145/3637882.3637886.
- Ille, N., Aurich, C., Erber, R., Wulf, M., Palme, R., Aurich, J., Von Lewinski, M., 2014. Physiological stress responses and horse rider interactions in horses ridden by male and female riders. *CEP* doi:10.3920/cep143001.

- Ille, N., Von Lewinski, M., Erber, R., Wulf, M., Aurich, J., Möstl, E., Aurich, C., 2013. Effects of the level of experience of horses and their riders on Cortisol release, heart rate and heart-rate variability during a jumping course. *Anim. welf.* doi:10.7120/09627286.22.4.457.
- Kikusui, T., 2017. Oxytocin bonds between human and dog. *Japanese Journal of Animal Psychology*, *The Japanese Journal of Animal Psychology* doi:10.2502/janip.67.1.1.
- Kotrschal, K., Schöberl, I., Bauer, B., Thibaut, A.M., Wedl, M., 2009. Dyadic relationships and operational performance of male and female owners and their male dogs. *Behavioural Processes* doi:10.1016/j.beproc.2009.04.001.
- Malinowski, K., Yee, C., Tevlin, J.M., Birks, E.K., Durando, M.M., Pournajafi-Nazarloo, H., Cavaola, A.A., McKeever, K.H., 2018. The Effects of Equine Assisted Therapy on Plasma Cortisol and Oxytocin Concentrations and Heart Rate Variability in Horses and Measures of Symptoms of Post-Traumatic Stress Disorder in Veterans. *Journal of Equine Veterinary Science* doi:10.1016/j.jevs.2018.01.011.
- Meinert, A., Deschner, T., Schaebs, F., Marshall-Pescini, S., Range, F., Gaugg, A., 2019. The Role of Oxytocin in the Dog–Owner Relationship. *Animals : an Open Access Journal from MDPI* doi:10.3390/ani9100792.
- Merkies, K., Sievers, A., Zakrajsek, E., MacGregor, H., Bergeron, R., Von Borstel, U.K., 2014. Preliminary results suggest an influence of psychological and physiological stress in humans on horse heart rate and behavior. *Journal of Veterinary Behavior* doi:10.1016/j.jveb.2014.06.003.
- Müller-Klein, A., Braun, M.N., Ferreira De Sá, D.S., Michael, T., Link-Dorner, U., Lass-Hennemann, J., 2024. A Relaxed Horse—A Relaxed Client? An Experimental Investigation of the Effects of Therapy Horses’ Stress on Clients’ Stress, Mood, and Anxiety. *Animals* doi:10.3390/ani14040604.
- Munsters, C.C., Visser, K.E., Van Den Broek, J., Sloet Van Oldruitenborgh-Oosterbaan, M.M., 2012. The influence of challenging objects and horse-rider matching on heart rate, heart rate variability and behavioural score in riding horses. *The Veterinary Journal* doi:10.1016/j.tvjl.2011.04.011.
- Odendaal, J., 2000. Animal-assisted therapy — magic or medicine? *Journal of Psychosomatic Research* doi:10.1016/S0022-3999(00)00183-5.
- Odendaal, J., Meintjes, R., 2003. Neurophysiological Correlates of Affiliative Behaviour between Humans and Dogs. *The Veterinary Journal* doi:10.1016/S1090-0233(02)00237-X.
- Patel, A., Foster, M., Torfs, T., Ahmmed, P., Castro, I., Holder, T., Bozkurt, A., 2021. Noncontact Electrophysiology Monitoring Systems for Assessment of Canine-Human Interactions. *2021 IEEE Sensors* doi:10.1109/SENSORS47087.2021.9639748.



- Peeters, M., Closson, C., Beckers, J.F., Vandenheede, M., 2013. Rider and Horse Salivary Cortisol Levels During Competition and Impact on Performance. *Journal of Equine Veterinary Science* doi:10.1016/j.jevs.2012.05.073.
- Pirrone, F., Ripamonti, A., Garoni, E.C., Stradiotti, S., Albertini, M., 2017. Measuring social synchrony and stress in the handler-dog dyad during animal-assisted activities: A pilot study. *Journal of Veterinary Behavior* doi:10.1016/j.jveb.2017.07.004.
- Von Lewinski, M., Biau, S., Erber, R., Ille, N., Aurich, J., Faure, J.M., Möstl, E., Aurich, C., 2013. Cortisol release, heart rate and heart rate variability in the horse and its rider: Different responses to training and performance. *The Veterinary Journal* doi:10.1016/j.tvjl.2012.12.025.
- Yoon, M., Jung, Y., 2025. The Effects of Human–Horse Interactions on Oxytocin and Cortisol Levels in Humans and Horses. *Animals : an Open Access Journal from MDPI* doi:10.3390/ani15070905.
