# Supplementary material for: Evidence of Physiological Co-Modulation During Human-Animal Interaction: A Systematic Review
Source: arXiv:2510.10559 ancillary file (2025-10-12)
Supplement: Supplementary file 5 [file S8_Physiological_Parameter_Synthesis_Table.pdf]

# Evidence of Physiological Co-Modulation During Human-Animal Interaction: A Systematic Review - Physiological Parameter Synthesis Table (S8)

| Physiological parameters                               | Animal specie(s)                                       | Interaction context                                                                                                                                     | Co-modulation outcome                                                                                                                    | Overall Risk of Bias                                 |
|--------------------------------------------------------|--------------------------------------------------------|---------------------------------------------------------------------------------------------------------------------------------------------------------|------------------------------------------------------------------------------------------------------------------------------------------|------------------------------------------------------|
| <b>Cardiac Activity</b>                                |                                                        |                                                                                                                                                         |                                                                                                                                          |                                                      |
| Heart Rate (n = 2) and Heart Rate Variability (n = 14) | Horse (n = 10)                                         | <ul style="list-style-type: none"> <li>• AAI/AAT 8 studies.</li> <li>• Non-Agonistic Sport: 2 studies.</li> </ul>                                       | <ul style="list-style-type: none"> <li>• Significant: 7 studies.</li> <li>• Partial: 2 studies.</li> <li>• Absent: 1 studies.</li> </ul> | High: ●●<br>Moderate to High: ●●●●<br>Moderate: ●●●● |
|                                                        | Dog (n = 6)                                            | <ul style="list-style-type: none"> <li>• Companionship: 6 studies.</li> </ul>                                                                           | <ul style="list-style-type: none"> <li>• Significant: 4 studies.</li> <li>• Partial: 1 studies.</li> <li>• Absent: 1 studies.</li> </ul> | High: ●<br>Moderate: ●●●●●                           |
| <b>Hormones</b>                                        |                                                        |                                                                                                                                                         |                                                                                                                                          |                                                      |
| Cortisol (n = 8)                                       | Horse (n = 3)                                          | <ul style="list-style-type: none"> <li>• AAI/AAT 1 study.</li> <li>• Agonistic Sport: 2 studies.</li> </ul>                                             | <ul style="list-style-type: none"> <li>• Significant: 1 studies.</li> <li>• Partial: 2 studies.</li> </ul>                               | High: ●<br>Moderate: ●●                              |
|                                                        | Dogs (n = 5)<br><i>(One study also included cats)</i>  | <ul style="list-style-type: none"> <li>• Companionship: 3 studies.</li> <li>• Agonistic Sport: 1 study.</li> <li>• Working Animals: 1 study.</li> </ul> | <ul style="list-style-type: none"> <li>• Significant: 2 studies.</li> <li>• Partial: 1 studies.</li> <li>• Absent: 2 studies.</li> </ul> | Moderate to High: ●<br>Moderate: ●●●●                |
| Oxytocin (n = 2)                                       | Dog (n = 2)<br><i>(One study also included wolves)</i> | <ul style="list-style-type: none"> <li>• Companionship: 2 studies.</li> </ul>                                                                           | <ul style="list-style-type: none"> <li>• Significant: 1 study.</li> <li>• Partial: 1 study.</li> </ul>                                   | Moderate: ●●                                         |

**Tabular synthesis based on Physiological Parameter — Part 1:**  
 The table illustrates the animal species enrolled, the interaction context, the Co-modulation outcomes, and the overall risk of bias for Cardiac Activity and Hormones categories of Physiological Parameter.  
 The risk of Bias categories for each study are colour-coded as: **Red** dots for High risk; **Orange** dots for Moderate to High risk; **Yellow** dots for Moderate risk.

| Physiological parameters                                            | Animal specie(s) | Interaction context                                                             | Co-modulation outcome                                                                                  | Overall Risk of Bias |
|---------------------------------------------------------------------|------------------|---------------------------------------------------------------------------------|--------------------------------------------------------------------------------------------------------|----------------------|
| <b>Multiparameter analysis</b>                                      |                  |                                                                                 |                                                                                                        |                      |
| Cardiac Activity and Cortisol (n = 3)                               | Horse (n = 2)    | <ul style="list-style-type: none"> <li>• AAT/AAI: 2 studies.</li> </ul>         | <ul style="list-style-type: none"> <li>• Significant: 1 study.</li> <li>• Partial: 1 study.</li> </ul> | Moderate: ●●         |
|                                                                     | Dog (n = 1)      | <ul style="list-style-type: none"> <li>• Companionship: 1 study.</li> </ul>     | <ul style="list-style-type: none"> <li>• Absent: 1 study.</li> </ul>                                   | Moderate: ●          |
| Cortisol and Oxytocin (n = 1)                                       | Dog (n = 1)      | <ul style="list-style-type: none"> <li>• Companionship: 1 study.</li> </ul>     | <ul style="list-style-type: none"> <li>• Partial: 1 study.</li> </ul>                                  | Moderate to High: ●  |
| Cardiac Activity, Cortisol and Oxytocin (n = 1)                     | Horse (n = 1)    | <ul style="list-style-type: none"> <li>• AAT/AAI: 1 study.</li> </ul>           | <ul style="list-style-type: none"> <li>• Significant: 1 study.</li> </ul>                              | Moderate: ●          |
| <b>Other physiological parameters</b>                               |                  |                                                                                 |                                                                                                        |                      |
| Testosterone ( <i>humans</i> ) and Cortisol ( <i>dogs</i> ) (n = 2) | Dog (n = 2)      | <ul style="list-style-type: none"> <li>• Agonistic Sport: 2 studies.</li> </ul> | <ul style="list-style-type: none"> <li>• Significant: 2 studies.</li> </ul>                            | Moderate: ●●         |
| Cortisol and Chromogranin A (n = 1)                                 | Dog (n = 1)      | <ul style="list-style-type: none"> <li>• Companionship: 1 study.</li> </ul>     | <ul style="list-style-type: none"> <li>• Significant: 1 study.</li> </ul>                              | Moderate: ●          |
| Hormonal, biochemical and haematological parameters (n = 1)         | Horse (n = 1)    | <ul style="list-style-type: none"> <li>• Agonistic Sport: 1 study.</li> </ul>   | <ul style="list-style-type: none"> <li>• Partial: 1 study.</li> </ul>                                  | Moderate: ●          |
| Breath rhythm (n = 1)                                               | Dog (n = 1)      | <ul style="list-style-type: none"> <li>• Companionship: 1 study.</li> </ul>     | <ul style="list-style-type: none"> <li>• Significant: 1 study.</li> </ul>                              | Moderate: ●          |
| Brain connectivity (n = 1)                                          | Dog (n = 1)      | <ul style="list-style-type: none"> <li>• Companionship: 1 study.</li> </ul>     | <ul style="list-style-type: none"> <li>• Significant: 1 study.</li> </ul>                              | Moderate: ●          |

#### Tabular synthesis based on Physiological Parameter — Part 2:

The table illustrates the animal species enrolled, the interaction context, the Co-modulation outcomes, and the overall risk of bias for Multiparameter analysis and Other physiological measures.

The risk of Bias categories for each study are colour-coded as: **Red** dots for High risk; **Orange** dots for Moderate to High risk; **Yellow** dots for Moderate risk.
